# Supplementary material for: Trajectory Advancement during Human-Robot Collaboration
Source: arXiv:1907.13445 source file (2019-07-31)
Supplement: Supplementary file 1 [file appendix.tex]

\section*{APPENDIX: Proof of Lemma~\ref{lemma-1}}
\label{proof:lemma-1}

\noindent \textbf{Proof:} The stability of $\dot{\widetilde{x}}$ can be analyzed by considering the following Lyapunov function: 

%\gabrisays{I strongly suggest to put the proof in an appendix in the end of the paper}

\begin{equation}
	\mathrm{V} = \frac{K_d}{2} \norm{\dot{x}(t) - \dot{x}_d(\psi)}^{2} + \frac{K_p}{2} \norm{\int_{0}^{t}(\dot{x}(t) - \dot{x}_d(\psi)) du}^{2}
	\label{eq:lyapunov-function}
\end{equation}

Now, on differentiating $\mathrm{V}$, we get: 
%\gabrisays{$K_d$ and $K_p$ are matrices so should stay in between $x^\top$ and $x$}

\begin{subequations}
	\begin{equation}
		\dot{\mathrm{V}} = \ \dot{\widetilde{x}}^T \ K_d \ \ddot{\widetilde{x}} + \ \int_{0}^{t} \dot{\widetilde{x}}^T du \ K_p \ \dot{\widetilde{x}} \notag		
	\end{equation}
	\begin{equation}
		\dot{\mathrm{V}} =  \dot{\widetilde{x}}^T \ K_d \ \ddot{\widetilde{x}} +  \ \dot{\widetilde{x}}^T \ K_p \int_{0}^{t}\dot{\widetilde{x}} \ du \  \notag
	\end{equation}
	\begin{equation}
        \dot{\mathrm{V}} = \dot{\widetilde{x}}^T \ [ K_d \ \ddot{\widetilde{x}} + K_p \ \int_{0}^{t}\dot{\widetilde{x}} \ du] \  \notag
	\end{equation}
\end{subequations}

\begin{equation}
	\dot{\mathrm{V}} = \dot{\widetilde{x}}^T \ [K_d \ \ddot{x}(t) + K_p \ \int_{0}^{t}\dot{\widetilde{x}} \ du - K_d \ \ddot{x}_d(\psi)]
	\label{Vdot}
\end{equation}

From the equation (\ref{eq:linear-jacobian-mapping}), on differentiating $\dot{x}(t)$ we get the following relation, %\gabrisays{maybe this one we can put it even after eq. 3}
\begin{equation}
	\ddot{x}(t) = J \dot{\nu} + \dot{J} \nu
	\label{eq:velocity-differentiaion}
\end{equation}

Using equation (\ref{eq:velocity-differentiaion}) in equation (\ref{Vdot}) we can write:
\begin{equation}
	\dot{\mathrm{V}} = \dot{\widetilde{x}}^T \ [ K_d \ [J \dot{\nu} + \dot{J} \nu] + K_p \ \int_{0}^{t}\dot{\widetilde{x}} \ du - K_d \ \ddot{x}_d(\psi)]
	\label{eq:vdot-final}
\end{equation}

The quantity $\dot{\nu}$ in equation (\ref{eq:vdot-final}) is the robot's acceleration that can be derived from the equations of motion as:
\begin{equation}
	\dot{\nu} = M^{-1}[B {\tau} + J^T f^* - h]
	\label{eq:robot-acceleration}
\end{equation}

where, $h = C(q,\nu) \nu + G(q)$. Now, the equation (\ref{eq:vdot-final}) can be written as,

\begin{subequations}
    \begin{multline}
        \dot{\mathrm{V}} = \dot{\widetilde{x}}^T \ [K_d \ J \ M^{-1}[B {\tau} + J_c^T f^* - h] + K_d \ \dot{J} \ v \\
                            + K_p \ \int_{0}^{t}\dot{\widetilde{x}} \ du - K_d \ \ddot{x}_d(\psi)] \notag
    \end{multline}
    \begin{multline}
        \dot{\mathrm{V}} = \dot{\widetilde{x}}^T  \ [K_d \  J \ M^{-1} \ B \ {\tau} + K_d \ J \ M^{-1} \ J_c^T f^* \\ 
                           + K_d \ \dot{J} \ v - K_d \  J \ M^{-1} \ h \\
                           + K_p \ \int_{0}^{t}\dot{\widetilde{x}} du - K_d \ \ddot{x}_d(\psi)] \notag
    \end{multline}
\end{subequations}

which can be written in compact form as,
\begin{equation}
    \dot{\mathrm{V}} = \dot{\widetilde{x}}^T \ [\mathbold{\Delta} \ \tau + \mathbold{\Omega} \ \mathrm{f}^* + \mathbold{\Lambda} + \mathbold{\beta}]
    \label{eq:vdot-compact}
\end{equation}

where, $ \mathbold{\Omega} = K_d J M^{-1} J_c^T \in \mathbb{R}^{6 \times \mathrm{n}}$. Now, on application of the robot torques from equation (\ref{equation:control-torques}), the equation (\ref{eq:vdot-compact}) becomes,

\begin{subequations}
    \begin{equation}
        \dot{\mathrm{V}} = \dot{\widetilde{x}}^T \ [\mathbold{\Omega} \ f^* - K \ \dot{\widetilde{x}}] \notag
    \end{equation}
    \begin{equation}
        \dot{\mathrm{V}} = - \dot{\widetilde{x}}^T \ K \ \dot{\widetilde{x}} \notag + \dot{\widetilde{x}}^T \ \mathbold{\Omega} \ f^* 
    \end{equation}
\end{subequations}

The stability of the system is ensured when $\dot{\mathrm{V}} \le 0$ which is ensured if,

\begin{subequations}
    \begin{equation}
        \dot{\widetilde{x}}^T \ \mathbold{\Omega} \ f^* \le 0 \notag
    \end{equation}
    \begin{equation}
        (\dot{x}(t) - \dot{x}_d(\psi))^T \ \mathbold{\Omega} \ f^* \le 0 \notag
    \end{equation}
    \begin{equation}
        (\dot{x}(t) - \partial_{\psi} x_d(\psi) \ \dot{\psi}) \ \mathbold{\Omega} \ f^* \le 0 \notag
    \end{equation}
    \begin{equation}
        \dot{x}(t) \ \ \mathbold{\Omega} \ \mathrm{f}^* \le \partial_{\psi} x_d(\psi) \ \dot{\psi} \ \mathbold{\Omega} \ f^* \notag
    \end{equation}
\end{subequations}

\begin{equation}
    \dot{\psi} \ge \frac{\dot{x}(t) \ \ \mathbold{\Omega} \ f^*}{\partial_{\psi} x_d(\psi)  \ \mathbold{\Omega} \ f^*}
    \label{eq:sdot-condition}
\end{equation}

The equation (\ref{eq:sdot-condition}) reflects the condition by which we can define the new parametrization $\psi$ to generate the reference parametric curve trajectory $x_d(\psi)$ that exploits the external interaction wrenches with the robot. The choice of $\dot{\psi}$ can be represented as:

\begin{equation}
    \dot{\psi} = max \{ 1, \frac{\dot{x}(t) \ \ \mathbold{\Omega} \ f^*}{\partial_{\psi} x_d(\psi)  \ \mathbold{\Omega} \ f^*} \}
    \label{eq:sdot-final-equation}
\end{equation}

where lower bound $1$ signifies that the new parametrization is equal to the time parametrization until any external wrench $f^*$ is applied such that it will help the robot's task. In such a case the value of $\dot{\psi}$ is greater than $1$. Accordingly, the integral of $\dot{\psi}$ stays linear until a \textit{favorable wrench} is applied to it and the value of $\psi$ increases and the reference trajectory generated is at a higher speed than the time parametrized trajectory with $\psi$ being linear. The value $\dot{\psi}$ is computed using equation (\ref{eq:sdot-final-equation}) and the reference trajectory is updated using the newly computed $\dot{\psi}$, under the influence of external forces, using the following relation: 

%\gabrisays{the proof seems ok but consider that I did not enter every single equation in details}

\begin{equation}
	x_d(\psi) = \int_{\psi(t_1)}^{\psi(t_2)} \partial_{\psi} x_d(\psi) \ \dot{\psi} \ du
\end{equation}

In addition, we can also set a velocity upper limit $\dot{\psi}_{upper}$ and update the $\dot{\psi}$ computation as,

\begin{equation}
    \dot{\psi} = min \{ \dot{\psi}_{upper}, max \{ 1, \frac{\dot{x}(t) \ \ \mathbold{\Omega} \ f^*}{\partial_{\psi} x_d(\psi)  \ \mathbold{\Omega} \ f^*}  \}\}
    \label{eq:sdot-final-equation-with-both-limits}
\end{equation}
